# Supplementary material for: Optimization at the Interface of Unitary and Non-unitary Quantum Operations in PCOAST
Source: arXiv:2305.09843 source file (2023-05-22)
Supplement: Supplementary file 1 [file appendix.tex]

\subsection{Ladder construction}

\note{\textbf{This appendix should be seen as internal notes. If we find it helpful, we should rephrase it providing a psudocode or a general procedure.}}

Here we explain how to measure commuting observables in the form of product of Paulis without re-preparing the state.
The non -trivial case is when the observables commute, but have different Pauli factors on single qubits.

It is easier to discuss a specific example since the generalization is straightforward.
Consider the set of two commuting observables: $\{ZZZ, ZXX\}$
The idea is measuring $ZZZ$ by collapsing the measured state in the eigenspaces of the observable and not by measuring each qubit in the computational basis.

Contrast these two cases:
\begin{itemize}
\item Direct measurement of $ZZZ$ returning one of the 2 eigenvalues, each associated with an eigenspace of dimension 4
\item Measure each qubit in the computational basis returning one of the 8 eigenvalues, each associated with an eigenspace of dimension 1
\end{itemize}
We do not want the latter since it corresponds to measuring the three observables $ZII$, $IZI$, $IIZ$ and not all of them commute with $ZXX$.
 
How can one measure $ZZZ$ directly?

\begin{lstlisting}
CNOT(0,1) 
CNOT(1,2)
Meas_Z(2) // this gives ZZZ
\end{lstlisting}
 
Then how to measure $ZXX$ without repreparing the state?
First of all, we revert to the initial frame:

\begin{lstlisting}
CNOT(1,2)
CNOT(0,1)
\end{lstlisting}

And then we measure $ZXX$:

\begin{lstlisting}
H(1)
H(2)
CNOT(0,1)
CNOT(1,2)
Meas_Z(2) // this gives ZXX
\end{lstlisting}
 
Note that the last measurement does not have the statistics of $\bra{\psi}ZXX\ket{\psi}$ but has the statistics of (apart from normalization):
$\bra{\psi} P_k \, ZXX \, P_k \ket{\psi}$
Where $P_k$ is the projector of the eigensubspace of $ZZZ$ for the outcome $k$ obtained in the $ZZZ$ measurement.
 However:
\begin{equation}
    \sum_k \bra{\psi} P_k \, ZXX \, P_k \ket{\psi} = \bra{\psi} ZXX \ket{\psi}
\end{equation}
since $ZXX$ and $ZZZ$ commute, and thus $ZXX$ commute with every $P_k$.
A proper treatment includes the probability of measuring $k$ and normalization, but they simplify.
